# Supplementary material for: First-principles investigations of the magnetic phase diagram of Gd$_{1-x}$Ca$_{x}$MnO$_{3}$
Source: arXiv:1810.08501 ancillary file (2019-04-08)
Supplement: Supplementary file 1 [file GCMO_HBH_supp_mat.pdf]

# Supplemental Material: First-principles investigations of the magnetic phase diagram of $Gd_{1-x}Ca_xMnO_3$

Hichem Ben Hamed,[1,*] Martin Hoffmann,[2,†] Waheed A. Adeagbo,[1] Arthur Ernst,[2,3] Wolfram Hergert,[1] Teemu Hynninen,[4] Kalevi Kokko,[5,6] and Petriina Paturi[4]

[1]*Institute of Physics, Martin Luther University Halle-Wittenberg, Von-Seckendorff-Platz 1, 06120 Halle, Germany*

[2]*Institute for Theoretical Physics, Johannes Kepler University Linz, Altenberger Straße 69, 4040 Linz, Austria*

[3]*Max Planck Institute of Microstructure Physics, Weinberg 2, 06120 Halle, Germany*

[4]*Wihuri Physical Laboratory, Department of Physics and Astronomy, University of Turku, FI-20014 Turku, Finland*

[5]*Department of Physics and Astronomy, University of Turku, FIN-20014 Turku, Finland*

[6]*Turku University Centre for Materials and Surfaces (MatSurf), Turku, Finland*

* hichem.ben-hamed@physik.uni-halle.de

† martin.hoffmann@jku.at

## A. Computational details

Our density functional theory (DFT) calculations were carried out with the projector augmented-wave method [1] as implemented in the Vienna *ab initio* simulation package (VASP) [2, 3]. The kinetic energy cutoff for the plane waves was set to 520 eV. Brillouin zone integrations were made using a Γ- centered k-point mesh sampling of $8 \times 8 \times 8$ k-points for the primitive unit-cell calculations and $4 \times 4 \times 4$ k-points for the supercell calculations. The local magnetic moments are obtained by using the standard method implemented in VASP. In this method the spin density is projected onto spheres around each atom. The method constructs the spheres in such a way that their overlap is minimized and the difference between the sum of the sphere volumes and the volume of the elementary cell is as little as possible (atomic sphere approximation). For GMO the radii are $R_{\mathrm{Gd}} = 1.588$ Å, $R_{\mathrm{Mn}} = 1.323$ Å and $R_{\mathrm{O}} = 0.82$ Å. The sum of the sphere volumina is 8 % smaller than the unit cell volume.

For GMO and CMO the relaxation of the structure is done in the following way: To avoid getting stuck in a local minimum in the complex determination of all atomic coordinates in the orthorhombic unit-cell, a three-steps geometrical relaxation was made within the conjugate gradient method. In the first step, only the cell shape and volume were allowed to relax, afterwards the internal coordinates were given the freedom to relax in the previously determined cell. Then a full relaxation of the system was made to minimize the inter atomic forces. A convergence threshold for the forces of 1 meV/Å was set.

## B. Electronic correlations

A crucial point in DFT calculations is the treatment of the exchange correlation potential. In this study, we considered four different functionals: namely Perdew-Burke-Ernzerhof (PBE) [4], its revised version for solids (PBEsol) [4], Perdew-Wang (PW91) [5] and Perdew-Zunger (PZ) [6]. An isotropically screened on-site Coulomb interaction [7] – the Hubbard $U$ correction – was additionally combined with each of the aforementioned functionals. The electronic and magnetic properties of the undoped sytems $\mathrm{GdMnO_3}$ (GMO) and $\mathrm{CaMnO_3}$ (CMO) were thoroughly investigated with the different functionals as well as varying the $U$ value from 0 eV to 8 eV (Table S1).

The choice of $U$ is the weak point in the treatment of electronic correlations with the DFT

TABLE S1. The variation of the band gap of GMO in the A-AFM order with the respect to the Hubbard $U$ corrected exchange correlation functional as explained in the text.

| $U$ | PBE | PBEsol | PW91 | PZ |
|---|---|---|---|---|
| 0 | 0.388 | 0.319 | 0.284 | 0.109 |
| 1 | 0.725 | 0.652 | 0.644 | 0.473 |
| 2 | 1.033 | 0.957 | 0.970 | 0.810 |
| 3 | 1.305 | 1.229 | 1.257 | 1.106 |
| 4 | 1.550 | 1.473 | 1.516 | 1.372 |
| 5 | 1.769 | 1.691 | 1.747 | 1.609 |
| 6 | 1.962 | 1.884 | 1.951 | 1.819 |
| 7 | 2.130 | 2.052 | 2.128 | 2.002 |
| 8 | 2.272 | 2.196 | 2.281 | 2.160 |

method including Hubbard $U$ corrections. The agreement of certain material properties with references values – be it from experiments or other theoretical sources – might be different for different $U$ values. One has always to find a compromise for the $U$ value describes all properties as good as possible, while the numerical effort with the Hubbard $U$ corrections is less than calculations with, e.g. hybrid functionals or the GW approximation. We took as reference properties the electronic band gap, the magnetic moment, and primarily the stability of the magnetic order.

Nevertheless, we stayed with the PBE exchange-correlation functional and $U = 2\,\text{eV}$ because higher values, as we will show later, lead to a wrong energetic order of the considered magnetic structures, with all studied functionals. We refer to this choice as PBE+$U$ in the main manuscript.

In [8], the band gap for GMO is found to be 0.45 eV for the PBE functional, 2.70 eV for a hybrid functional (HSE) and 1.87 eV in the framework of the $G_0W_0$ approximation. Thus, HSE and $G_0W_0$ results are in good agreement with experimental values given in [8]. Table S1 shows, that an increase of $U$ to 8.0 eV allows to get similar band gaps like in HSE or $G_0W_0$. We have to stay with $U = 2.0\,\text{eV}$ to get correct magnetic properties, accepting an underestimation of the gap.

We restrict our GCMO investigation to the PBE+$U$ method. It should be noted here, that the four studied exchange correlation functionals lead to comparable band gaps within the A-AFM magnetic order.

### C. Magnetic moments

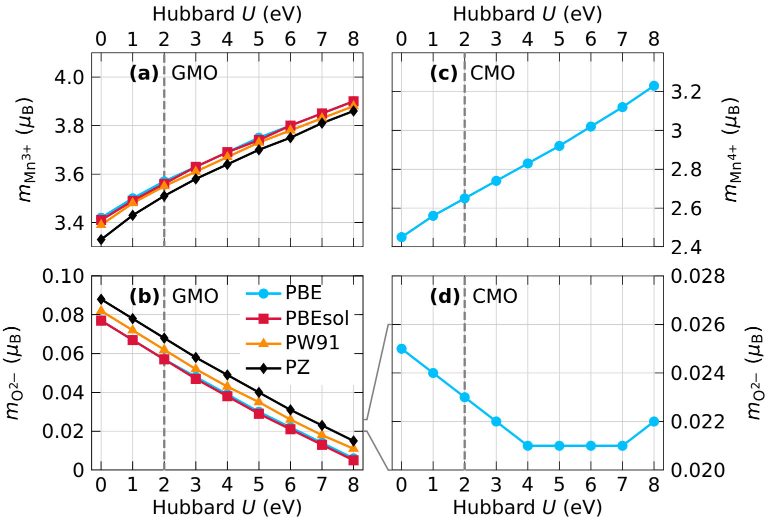


FIG. S1. Magnetic moments in dependence on exchange correlation functional and Hubbard $U$ correction. (a),(b) magnetic moments for $Mn^{3+}$, $O^{2-}$ in GMO, (c),(d) magnetic moments for $Mn^{4+}$, $O^{2-}$ in CMO, respectively. (For CMO only calculations with PBE functional were done). The gray dashed line indicates the choice of $U = 2\,\text{eV}$. The lines between (b) and (d) just visualize the big difference in scale. Note that the magnetic moments at the oxygen ions are so small that the accuracy is restricted to the output precision in VASP (see text).

For each magnetic state considered in the paper, we get an integer moment for the unit cell, i.e. it is 16 for GMO in the FM state and 0 in the A-AFM. The 3$d$ Mn wavefunctions are not totally located inside the corresponding sphere. This leads to a polarization of the surrounding oxygen atoms and the magnetic moment of the Mn atoms is less than 4 $\mu_B$. In the density of states (DOS), this is represented by the hybridization of the O 2$p$ and the Mn 3$d$ states (see Fig. S2) . The localization of the Mn 3$d$ states depends on the $U$-value. Fig. S1 reveals the change of the moments in dependence on $U$. An increasing $U$ leads to a stronger localization of the Mn 3$d$ wavefunction, i.e. the moment increases. In parallel, the calculated magnetic moments at the oxygen ions decrease in GMO. In CMO, those moments

and their variation with $U$ are so small, that it looks like a piece-wise behavior of $m_{\mathrm{O}^{2-}}$. There is presumably no physical reason for that behavior but only the restricted precision in the output of magnetic moments in VASP (rounded up to 0.001 digits).

All studied exchange correlation functionals converge to similar magnetic moments for both materials – GMO and CMO (Fig. S1). Increasing the correlation corrections $U$ raises the magnetic moments at the Mn ions, while the magnetic moments at the oxygen ions become smaller: The Mn $d$ states become more localized.

### D. Densities of states

Fig. S2 presents the densities of states for the GCMO series. For GMO the DOS corresponds to the A-AFM mangetic ground state. In case of CMO the DOS corresponds to the G-AFM state. For concentrations $0 < x < 1$ we get an half-metallic behaviour. The number of states in the spin-up channel near $E_\mathrm{F}$ decreases with increasing $x$.

### E. Determination of exchange parameters

The total energy of each magnetic configuration (noted with $X$) can be written as

$$E_X = E_0 - \frac{S^2}{2}\left[n_x\sigma_1\sigma_2 J_x + n_z\sigma_1\sigma_3 J_z + n_{xz}\sigma_1\sigma_4 J_{xz}\right] , \tag{1}$$

wherein the $\sigma_i$ ($i = 1, ..., 4$) represent the spin orientation on the $i$-th site, having a value of either $+1$ for spin up or $-1$ for spin down. The numbers $n_x$, $n_z$, and $n_{xz}$ count the number of $J_x$, $J_z$, and $J_{xz}$ exchange parameters in the considered cell, respectively. In the unit cell (Fig. 2 of the paper), each Mn has, e.g., 4 interactions with nearest neighbors ($J_x$), which results in $n_x = 16$. Similary, each Mn has $2J_z$ interactions and $8J_{xz}$ with its neighbors, which leads to $n_z = 8$ and $n_{xz} = 32$.

The total energies of $Gd_{1-x}Ca_xMnO_3$ for all considered magnetic structures are shown in Table S2. The lowest energy for each concentration is taken as reference. A strong competition between various AFM orders can be observed for $x > 1/2$ (Table S2). Those energies are the basis for the calculation of the exchange parameters.

The energies of FM, A-AFM, C-AFM, and G-AFM, and FiM structures are used for the calculation of the exchange parameters, following the recipe given in [8]. In principle, also

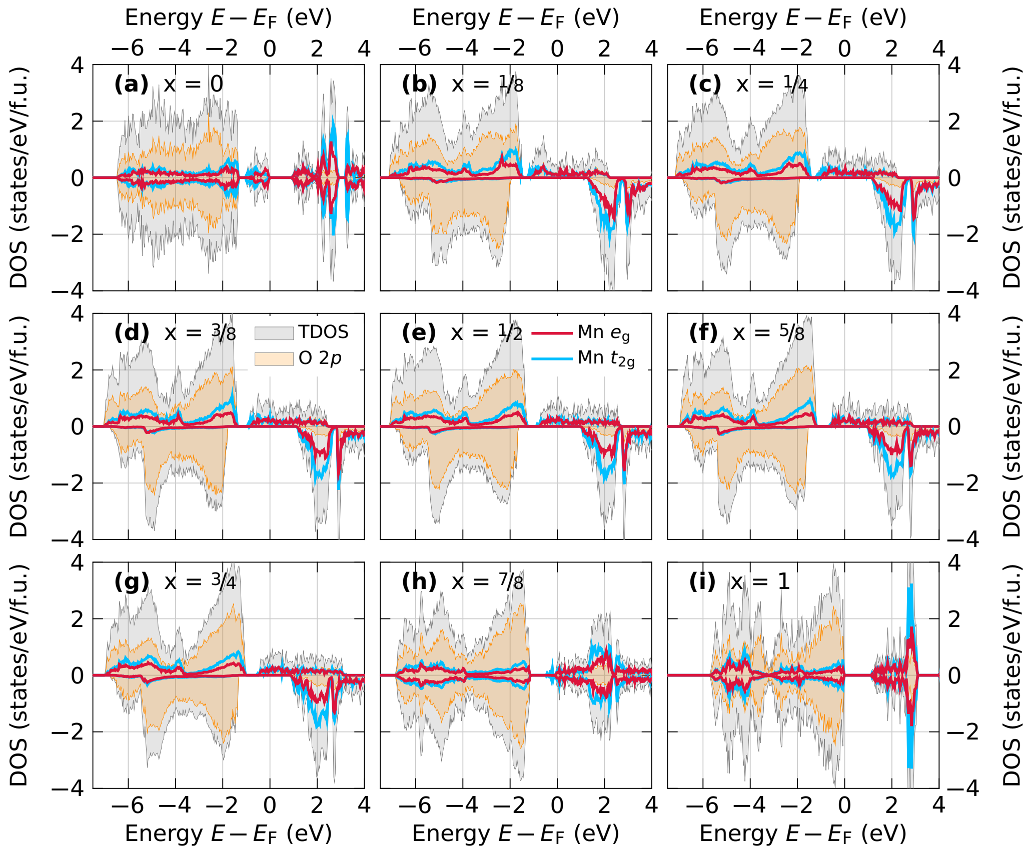


FIG. S2. DOS for the $Gd_xCa_{(1-x)}MnO_3$ series. Positive values represent the spin up channel, while negative values stand for spin down. Total DOS is given in gray, the partial DOS of the O $2p$ states in yellow. The Mn $e_\mathrm{g}$ and $t_{2\mathrm{g}}$ states are plotted in red and blue, respectively.

more energies could be included in the fit, but the large unit cells (see Fig. 1 of the paper) complicate the equations to find the exchange interactions without a clear gain in accuracy. Thus, a set of four linear equations is considered in a least square fit for the three $J$'s. This can be written as $\underline{\underline{M}}\,\boldsymbol{J} = \boldsymbol{E}$. The matrix $\underline{\underline{M}}$ contains the coefficients of the linear equations, $\boldsymbol{J}$ is the vector of the exchange parameters and $\boldsymbol{E}$ is the vector containing the *ab initio* energies.

In order to double check the obtained exchange parameters and estimate the error of the fitting procedure, we have also used a second method: By using only 4 instead of 5 magnetic configurations, we obtain 4 sets of three linear independent equations, which determine the $J_{ij}$ parameter. The 4 sets result always in two different values for $J_x$, $J_z$, and $J_{xz}$, which are different from the values obtained from the least square fit described above. However, the calculated mean values over the four sets of exchange parameters lead to the exact same

TABLE S2. Total energies per f.u. for $Gd_{1-x}Ca_xMnO_3$ in meV.

| | 0 | 0.125 | 0.25 | 0.375 | 0.5 | 0.625 | 0.75 | 0.875 | 1 |
|---|---|---|---|---|---|---|---|---|---|
| A-AFM | 0.00 | 29.01 | 49.090 | 42.85 | 37.91 | 24.55 | 16.57 | 0.00 | 11.77 |
| C-AFM | 29.3 | 96.56 | 147.25 | 179.55 | 185.4 | 79.07 | 35.31 | 11.87 | 4.624 |
| G-AFM | 30.9 | 99.68 | 198.16 | 360.88 | 211.7 | 126.74 | 74.75 | 28.69 | 0.00 |
| FM | 4.09 | 0.00 | 0.00 | 0.00 | 0.00 | 0.00 | 0.00 | 2.08 | 32.10 |
| D-AFM | 19.9 | 78.75 | 124.98 | 138.51 | 118.4 | 143.41 | 38.33 | 18.57 | 8.618 |
| E-AFM | 9.27 | 66.66 | 116.44 | 185.25 | 113.9 | 173.03 | 63.62 | 28.40 | 8.315 |
| H-AFM | 8.17 | 52.73 | 85.540 | 98.14 | 85.00 | 71.47 | 45.64 | 20.14 | 14.66 |
| I-AFM | 8.10 | 50.76 | 90.342 | 101.54 | 124.3 | 77.19 | 63.43 | 34.64 | 17.62 |
| CE-AFM | 12.8 | 145.0 | 120.88 | 122.30 | 94.10 | 69.75 | 44.23 | 15.31 | 5.146 |
| FI | 14.0 | 57.24 | 158.74 | 133.70 | 81.65 | 71.46 | 20.21 | 4.84 | 11.56 |

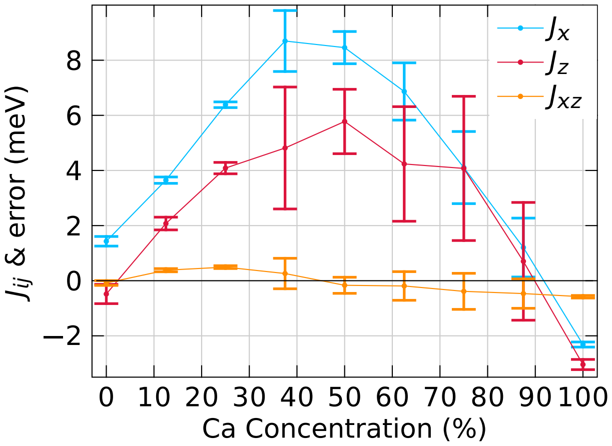


FIG. S3. The three Heisenberg exchange interactions for GCMO with error bars from the fitting procedure (see text).

values obtained with the least square fit, while two different $J_{ij}$ parameter within each set give a lower and upper bound of the averaged $J_{ij}$ parameter. This error is small for $J_x$, but becomes rather large for $J_{xz}$ (see Fig. S3). Hence, $J_x$ is much less sensitive to the choice of magnetic configuration than the other two magnetic exchange parameter. The error becomes in particular larger for the concentration range of $c \geq 0.375$ to $\leq 0.875$. This fact could also

play a part in the observed differences between the theoretical and experimental results for the Curie temperature.

TABLE S3. Exchange interactions for $Gd_{1-x}Ca_xMnO_3$ in meV derived from the total energies.

| x | 0.000 | 0.125 | 0.250 | 0.375 | 0.500 | 0.625 | 0.750 | 0.875 | 1.000 |
|---|---|---|---|---|---|---|---|---|---|
| $S$ | 2.000 | 1.938 | 1.875 | 1.813 | 1.75 | 1.688 | 1.625 | 1.563 | 1.500 |
| $J_x$ | 1.430 | 3.648 | 6.385 | 8.697 | 8.457 | 6.866 | 4.105 | 1.203 | -2.316 |
| $J_z$ | -0.484 | 2.075 | 4.086 | 4.815 | 5.777 | 4.236 | 4.074 | 0.703 | -3.041 |
| $J_{xz}$ | -0.083 | 0.382 | 0.493 | 0.260 | -0.166 | -0.190 | -0.386 | -0.466 | -0.582 |
| $J_{\mathrm{eff}}$ | -0.816 | 3.603 | 6.058 | 5.855 | 5.113 | 3.476 | 2.530 | -1.161 | -5.369 |

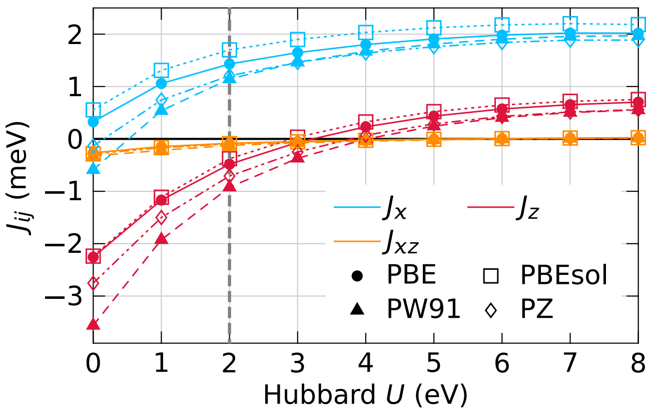


FIG. S4. The three Heisenberg exchange interactions in dependence of the exchange correlation functional and the Hubbard U correction in $GdMnO_3$. The gray dashed line indicates the choice of $U = 2\,\mathrm{eV}$ in this work.

The different exchange correlation functionals lead to comparable results for the exchange parameters. In all cases, the spins in GMO order ferromagnetically between $U = 3\,\mathrm{eV}$ to $4\,\mathrm{eV}$ due to the dominating in-plane ($J_x$) and out-of-plane ($J_z$) nearest neighbor interaction (Fig. S4). We note that we obtain with the PBE+$U$ setup already similar results for the exchange parameters as presented in the work of Kováčik *et al.* [8], although they calculated the exchange interactions constants for the rare earth manganite series $R\mathrm{MnO}_3$ by means of hybrid functionals and the GW approximation. These two methods are computationally

demanding and were therefore excluded for our calculations because of the large supercells at several different Ca concentrations.

Besides the exchange parameters $J_x$, $J_z$, $J_{xz}$ and the effective spin moment corresponding to each Ca concentration $x$ also the effective out-of-plane interaction $J_{\mathrm{eff}} = J_z + 4J_{xz}$ is given in Table S3. In the region $0.0 < x \leq 0.5$ the exchange parameters $J_x$ and $J_{\mathrm{eff}}$ describe a ferromagnetic structure. $J_{\mathrm{eff}}$ decreases with increasing $x$, describing a tendency to an antiferromagnetic structure.

### F. Special quasi random structure generation

As the special quasi random structure (SQS) per Ca concentration is that SQS selected, which has the the smallest value for its objective function. The latter is thereby a measure of the match between the correlation function of the SQS candidate and the completely random structure and reads [9]

$$\mathcal{F} = -L + \sum_{\alpha \in \mathcal{A}} \left| \Delta\rho_\alpha \left( \varSigma \right) \right| ,$$

wherein $L$ is the largest diameter where a perfect match in the pair correlation function is found, $\varSigma$ is the occupation of the sublattice, and $\mathcal{A}$ is a set of clusters $\alpha$. The difference between correlations of the SQS candidate and those of a random structure is noted as $\Delta\rho$. A typical variation run of the structural occupation for $x = 0.5$ is depicted in Fig. S5.

Only the pair correlation functions of the SQS at $x = 1/4$, $1/2$, and $3/4$, match perfectly those of the random distribution (Table S4). The correlation functions as well as the objective functions for $x$ are the same at $1 - x$ (except of a different sign). Nevertheless, they do not have necessarily the same atomic distribution. As an example, the SQS structure for $x = 3/4$ (see Fig. S6) is not a simple substitution of one element (Gd or Ca) by another element (Ca or Gd) in the SQS structure of $x = 1/4$. The objective function becomes larger when the corresponding structure is more disordered. It tends towards $-\infty$ in the case of $x = 1/2$.

In order to get an impression of the involved energy scale, we calculated the total energies for the different SQS candidates presented in Fig S4 ($x = 0.5$) with VASP and compared them with each other. The overall variation of the total energy of one SQS to another one differs by maximal 9 meV/f.u.. This energy scale is comparable with that of a careful

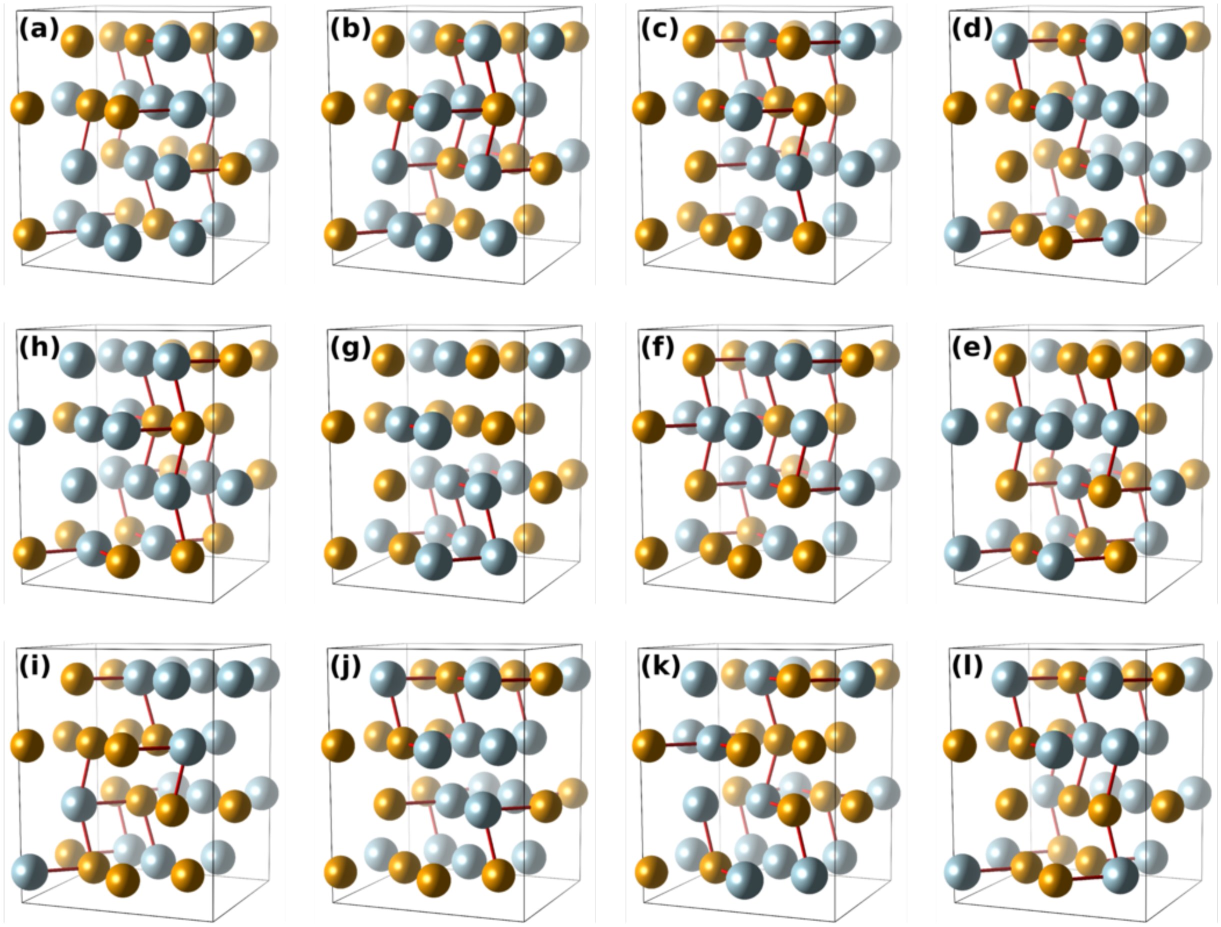


FIG. S5. The different SQS structures of $Gd_{1-x}Ca_xMnO_3$ at $x = 0.5$ in the 32 f.u. supercell considered in a typical MCSQS run [9]. The supercell shape is fixed. The objective function becomes smaller from the upper left to the lower right structure. The colored balls depict Gd (golden) and Ca (gray) ions. For the sake of clarity, Mn and O sites are omitted. The shortest bond lengths linking two different chemical elements (Gd or Ca) are highlighted by dark red lines. For the final SQS structure at $x = 0.5$ see Fig. S6.

comparison between SQS with 16 and 32 atoms, showing energy differences of 2 meV/atom [10]. Hence, there might be several equivalent realizations of the minimal correlation function possible, but the typical energy scale for them is rather small.

---

[1] G. Kresse and D. Joubert, Phys. Rev. B **59**, 1758 (1999).

[2] G. Kresse and J. Furthmüller, Comp. Mater. Sci. **6**, 15 (1996).

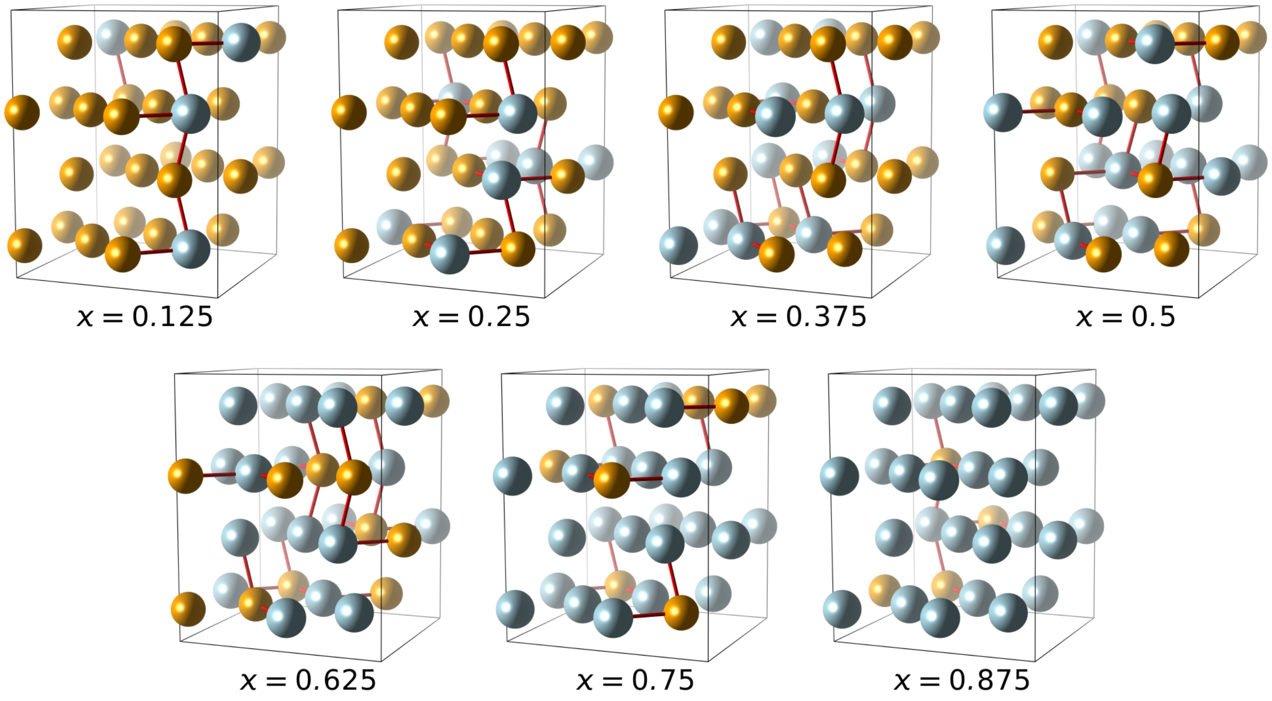


FIG. S6. The final SQS structures of $Gd_{1-x}Ca_xMnO_3$ considered in this study at different $x$. The shortest bond lengths linking two different chemical elements (Gd or Ca) are highlighted by dark red lines.


[3] G. Kresse and J. Furthmüller, Phys. Rev. B **54**, 11169 (1996).

[4] J. P. Perdew, K. Burke, and M. Ernzerhof, Phys. Rev. Lett. **77**, 3865 (1996).

[5] J. P. Perdew and Y. Wang, Phys. Rev. B **45**, 13244 (1992).

[6] J. P. Perdew and A. Zunger, Phys. Rev. B **23**, 5048 (1981).

[7] S. L. Dudarev, G. A. Botton, S. Y. Savrasov, C. J. Humphreys, and A. P. Sutton, Phys. Rev. B **57**, 1505 (1998).

[8] R. Kováčik, S. S. Murthy, C. E. Quiroga, C. Ederer, and C. Franchini, Phys. Rev. B **93**, 075139 (2016).

[9] A. van de Walle, P. Tiwary, M. de Jong, D. Olmsted, M. Asta, A. Dick, D. Shin, Y. Wang, L.-Q. Chen, and Z.-K. Liu, Calphad **42**, 13 (2013).

[10] D. Shin, R. Arróyave, Z.-K. Liu, and A. Van de Walle, Phys. Rev. B **74**, 024204 (2006).

TABLE S4. The difference between the correlation functions of the SQS candidates and the target disordered state for each concentration of GCMO, different numbers ($n$) of interaction partners (pair-, three- or four interactions), and different corresponding distances ($r$). The optimal SQS has the same correlation functions as the targeted disordered state, i.e, the difference is zero. The last row shows the objective function value.

| $n$ | $r$ | Concentrations $x$ | | | | | | |
|---|---|---|---|---|---|---|---|---|
| | | 0.125 | 0.25 | 0.375 | 0.5 | 0.625 | 0.75 | 0.875 |
| 2 | 3.8541 | -0.0625 | 0.0000 | -0.0625 | 0 | -0.0625 | 0.0000 | -0.0625 |
| 2 | 3.8541 | -0.0625 | 0.0000 | -0.0625 | 0 | -0.0625 | 0.0000 | -0.0625 |
| 2 | 3.8678 | -0.0625 | 0.0000 | -0.0625 | 0 | -0.0625 | 0.0000 | 0.0625 |
| 2 | 4.1262 | 0.0625 | 0.0000 | -0.0625 | 0 | -0.0625 | 0.0000 | -0.0625 |
| 2 | 4.9751 | 0.0625 | 0.0000 | -0.0625 | 0 | -0.0625 | 0.0000 | 0.0625 |
| 2 | 4.9751 | 0.0625 | 0.0000 | -0.0625 | 0 | -0.0625 | 0.0000 | 0.0625 |
| 2 | 5.3449 | -0.0625 | 0.0000 | -0.0625 | 0 | -0.0625 | 0.0000 | -0.0625 |
| 2 | 5.9375 | -0.0625 | 0.0000 | -0.0625 | 0 | -0.0625 | 0.0000 | -0.0625 |
| 2 | 6.0658 | -0.0625 | 0.0000 | -0.0625 | 0 | -0.0625 | 0.0000 | -0.0625 |
| 2 | 6.0658 | -0.0625 | 0.0000 | -0.0625 | 0 | -0.0625 | 0.0000 | -0.0625 |
| 2 | 6.1699 | -0.0625 | 0.0000 | -0.0625 | 0 | -0.0625 | 0.0000 | -0.0625 |
| 2 | 6.1699 | -0.0625 | 0.0000 | -0.0625 | 0 | -0.0625 | 0.0000 | -0.0625 |
| 2 | 6.4309 | -0.0625 | 0.0000 | -0.0625 | 0 | -0.0625 | 0.0000 | -0.0625 |
| 2 | 6.4309 | -0.0625 | 0.0000 | -0.0625 | 0 | -0.0625 | 0.0000 | -0.0625 |
| 3 | 4.9751 | -0.0781 | 0.1250 | 0.0156 | 0 | -0.0156 | 0.1250 | -0.0468 |
| 3 | 4.9751 | 0.0468 | -0.1250 | 0.0156 | 0 | -0.0156 | 0.1250 | 0.0781 |
| 3 | 4.9751 | 0.0468 | 0.1250 | 0.0156 | 0 | -0.0156 | 0.1250 | 0.0781 |
| 3 | 4.9751 | -0.0781 | 0.1250 | 0.0156 | 0 | -0.0156 | -0.1250 | -0.0468 |
| 3 | 5.3449 | 0.0468 | 0.1250 | 0.0156 | 0 | -0.0156 | -0.1250 | -0.0468 |
| 3 | 5.3449 | 0.0468 | 0.1250 | 0.0156 | 0 | -0.0156 | -0.1250 | -0.0468 |
| 3 | 5.3449 | -0.0781 | -0.1250 | 0.0156 | 0 | -0.0156 | -0.1250 | 0.0781 |
| 3 | 5.3449 | -0.0781 | 0.1250 | 0.0156 | 0 | -0.0156 | 0.1250 | 0.0781 |
| 4 | 5.3449 | 0.0585 | -0.0625 | -0.0039 | 0 | -0.0039 | -0.0625 | 0.0585 |
| 4 | 5.3449 | 0.0585 | -0.0625 | -0.0039 | 0 | -0.0039 | -0.0625 | 0.0585 |
| $\mathcal{F}$ | | -2.9378 | -5.1940 | -2.9580 | $-\infty$ | -2.9580 | -5.1940 | -2.9378 |
